# Supplementary material for: Tricking AI chips into Simulating the Human Brain: A Detailed Performance Analysis
Source: arXiv:2301.13637 source file (2023-01-31)
Supplement: Supplementary file 1 [file 999-supplement.tex]

\begin{figure*}[t!]
    \centering
    \includegraphics[width=\textwidth]{img/supplementfigallsims-3.pdf}
    \caption{Runtime performance (lower is better), comparison between CPU baseline, GPU and AI chips. For scale, the mouse and human inferior olive are shown as running in realtime in the figures.}
\end{figure*}
